# Supplementary material for: Second-order Approximation of Minimum Discrimination Information in Independent Component Analysis
Source: arXiv:2111.15060 source file (2021-11-30)
Supplement: Supplementary file 1 [file supplemental_materials.pdf]

# Supplementary Materials for Submission "Second-order Approximation of Minimum Discrimination Information in Independent Component Analysis"

## 1 Details of experiments with simulated signals

### 1.1 Details of 18 distributions

Page 4, Column 1, Section IV, Subsection A, Fig1
The details of the sources' distributions used in the first experiment are shown in Figure 1.

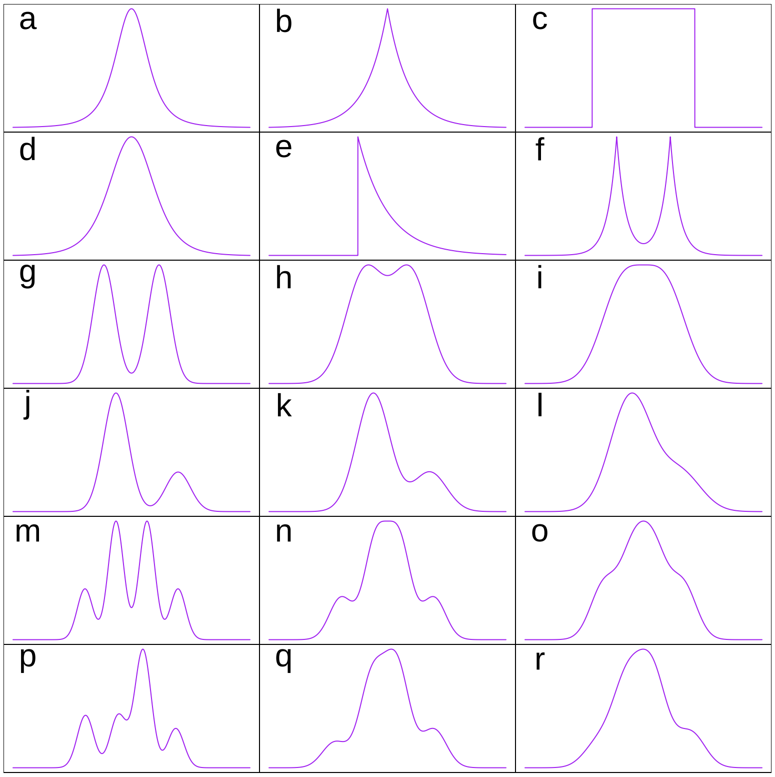


Figure 1: Probability density functions of sources: $(a)$ Student with 3 degrees of freedom; $(b)$ double exponential; $(c)$ uniform; $(d)$ Student with 5 degrees of freedom; $(e)$ exponential; $(f)$ mixture of two double exponentials; $(g)-(h)-(i)$ symmetric mixtures of two Gaussians: multimodal, transitional and unimodal; $(j)-(k)-(l)$ nonsymmetric mixtures of two Gaussians, multimodal, tran- sitional and unimodal; $(m)-(n)-(o)$ symmetric mixtures of four Gaussians: mul- timodal, transitional and unimodal; $(p)-(q)-(r)$ nonsymmetric mixtures of four Gaussians: multimodal, transitional and unimodal.

### 1.2 Details of 18 two dimensional experiments

Page 4, Column 1, Section IV, Subsection B
The Amaric metrics and CPU elapsed time are recorded in Table 1, Table 2. Since the public EFICA package was implemented on Matlab development platform and other ICA algorithms we used were implemented on R development platform, it might not be appropriate to compare the CPU elapsed time between EFICA and other ICA algorithms (we denoted the EFICA's CPU elapsed time with superscript $^*$).

$FastICA$ works well only when its single nonlinear function is close to the unknown sources' distribution, otherwise its separation performance or negentropy estimation might degenerate due to the unwanted density mismatching. As can be seen in Figure 1, F-G0 and F-G1 perform well in symmetric distributions (f, g, h, i) thanks to their symmetric nonlinear functions (F-G0: $G0 = \frac{y_i^4}{4}$, F-G1: $G1 = \log cosh(y_i)$ ) used in negentropy estimation (density matching), whereas their separation performance deteriorates in the cases of nonsymmetric or nontrivial distributions (j, k, l, p, q, r, n). Compared with the single nonlinear function used in F-G0 and F-G1, the nonparametric estimation used in PICA or several nonlinear functions used in MICA are more flexible in these nontrivial cases. Although PICA performed best in general (thanks to its flexible nonparametric estimation concerning negentropy), its CPU elapsed time is demanding. The CPU elapsed time required by MICA (88.89 ms) is less than PICA (556.11 ms), as a result of transforming a sequence of IRLS (in PICA) into a single weighted least squares (in MICA).

Table 1: Amari metrics for two-component ICA with 1000 samples .For each pdf (from a to r), averages over 100 replicates are presented.

| pdfs | F-G0 | F-G1 | PICA | MICA | WICA | EICA |
|---|---|---|---|---|---|---|
| a | 4.06(±4.06) | 2.47(±1.7) | 2.47(±1.83) | 3.29(±8.24) | 13.19(±17.61) | 3.54(±2.82) |
| b | 4.12(±3.22) | 2.92(±1.47) | 2.62(±1.29) | 3.48(±2.2) | 33.31(±25.76) | 2.03(±1.36) |
| c | 1.56(±0.93) | 1.81(±1.06) | 3.44(±12.86) | 5.59(±15.84) | 56.45(±27.76) | 1.42(±1.22) |
| d | 5.1(±3.97) | 3.78(±2.45) | 3.84(±2.48) | 4.8(±3.75) | 20.27(±21.07) | 6.42(±5.42) |
| e | 3.94(±3.76) | 3.14(±1.87) | 1.6(±0.91) | 6.32(±12.37) | 30.01(±24.74) | 3.27(±2.11) |
| f | 2.62(±1.72) | 1.7(±0.97) | 27.11(±42.53) | 1.94(±1.42) | 47.93(±28.39) | 6.16(±7.54) |
| g | 1.49(±0.84) | 1.44(±0.85) | 23.55(±40.63) | 4.5(±6.2) | 66.11(±24.74) | 3.61(±2.37) |
| h | 4.23(±3.02) | 3.32(±2.24) | 4.94(±12.45) | 4.8(±7.7) | 50.31(±29.29) | 4.18(±3.14) |
| i | 6.75(±4.76) | 5.87(±4.44) | 7.63(±8.36) | 8.87(±9.44) | 46.46(±28.5) | 6.02(±4.22) |
| j | 7.52(±8.11) | 44.33(±41.06) | 5.68(±17.99) | 1.76(±1.04) | 37.97(±28.9) | 68.7(±35.46) |
| k | 17.47(±20.53) | 34.22(±34.17) | 2.08(±1.35) | 2.2(±1.39) | 41.98(±28.4) | 33.2(±33.37) |
| l | 28.44(±27.52) | 32.06(±27.38) | 4.03(±2.46) | 5.3(±9.13) | 42.89(±26.42) | 30.67(±27.77) |
| m | 3.49(±2.25) | 5.06(±3.38) | 4.77(±16.37) | 12.17(±14.97) | 53.46(±29.39) | 3.48(±2.23) |
| n | 14.67(±15.28) | 47.31(±27.39) | 10.13(±23.51) | 38.1(±26.83) | 50.46(±25.77) | 48.6(±26.51) |
| o | 4.78(±2.8) | 6.68(±4.28) | 6.71(±13.26) | 11.01(±14.14) | 44.69(±28.77) | 5.51(±3.56) |
| p | 3.8(±2.79) | 15.67(±15.49) | 2.33(±8.97) | 4.09(±3.18) | 46.19(±27.67) | 8.37(±15.7) |
| q | 41.18(±27.54) | 23.46(±26.62) | 5.26(±13.14) | 17.63(±22.69) | 43.2(±27.64) | 27.65(±26.6) |
| r | 24.98(±23.38) | 44.55(±28.95) | 6.39(±10.62) | 12.38(±13.41) | 49.51(±28.03) | 43.72(±28.27) |

### 1.3 Details of high dimensional experiments

We included the high dimensional experiments (originally shown in the first submission) in the supplementary materials due to the page limit of "IEEE Signal Processing Letters". As can be seen in Table 3 and Table 4, PICA performed best with the longest running time (thanks to its flexible nonparametric estimation, whereas a sequence of IRLS are required to solved), and MICA have the second lowest Amari metrics with the acceptable CPU elapsed time (thanks to the adding more nonlinear functions in the negentropy estimation without destroying the efficient fixed-point method compared with F-G0 and F-G1).

Table 2: CPU elapsed time (ms) for two-component ICA with 1000 samples .For each pdf (from a to r), averages over 100 replicates are presented.

| pdfs | F-G0 | F-G1 | PICA | MICA | WICA | EICA |
|---|---|---|---|---|---|---|
| a | 6.83(±5.87) | 9.34(±6.15) | 883.67(±385.18) | 72.97(±31.11) | 5.23(±4.75) | 7.4*(±5.79*) |
| b | 8.05(±4.03) | 8.39(±5.48) | 510.72(±210.95) | 54.28(±16.98) | 4.69(±1.53) | 5*(±5.41*) |
| c | 7.04(±5.69) | 5.77(±2.94) | 442.81(±201.58) | 78.28(±38.45) | 4.67(±1.1) | 5.1*(±5.02*) |
| d | 8.55(±6.81) | 10.02(±6.47) | 740.89(±267.51) | 65.94(±29.66) | 4.71(±0.94) | 5.5*(±5.57*) |
| e | 7.66(±3.67) | 10.33(±7.4) | 435.1(±193.75) | 77.59(±30.53) | 4.73(±2.11) | 5.2*(±5.41*) |
| f | 5.85(±2.55) | 4.62(±2.43) | 357.74(±173.23) | 56.24(±32.51) | 4.79(±1.57) | 4.5*(±5*) |
| g | 5.64(±3.7) | 4.6(±2.65) | 372.12(±202.82) | 105.74(±35.33) | 4.76(±1.75) | 4.4*(±4.99*) |
| h | 9.75(±6.77) | 7.69(±4.87) | 611.35(±201.57) | 104.21(±29.99) | 4.56(±1.04) | 3.3*(±4.93*) |
| i | 11.93(±7.34) | 11.14(±7.62) | 668.38(±149.08) | 111.74(±22) | 4.61(±1.44) | 4.6*(±5.21*) |
| j | 10.51(±6.21) | 12.6(±8.01) | 373.46(±214.14) | 35.31(±16.14) | 4.55(±0.67) | 4.8*(±5.22*) |
| k | 12.35(±7.48) | 14.87(±8.34) | 402.61(±205.03) | 45.31(±25.61) | 4.67(±1.51) | 3.8*(±5.46*) |
| l | 13.03(±8.06) | 15.71(±7.65) | 593.5(±198.13) | 60.85(±29.8) | 4.76(±1.78) | 4.9*(±5.59*) |
| m | 9.21(±4.83) | 9.78(±5.99) | 502.49(±253.81) | 128.87(±22.69) | 4.96(±2.3) | 5*(±5.95*) |
| n | 14.26(±7.52) | 17.99(±8.74) | 644.78(±206.62) | 127.16(±20.71) | 5.08(±1.76) | 5.2*(±5.94*) |
| o | 9.7(±6.33) | 11.56(±8.27) | 688.88(±169.91) | 127.19(±30.57) | 5.27(±2.82) | 3.8*(±4.88*) |
| p | 10.27(±6.84) | 14.06(±7.76) | 411.55(±198.01) | 66.94(±35.25) | 4.97(±1.75) | 3.8*(±4.88*) |
| q | 11.96(±10.44) | 14.98(±9.36) | 661.84(±222.94) | 138.21(±42.57) | 5.14(±2.23) | 5*(±5.6*) |
| r | 15.81(±8.99) | 17.66(±9.11) | 734.84(±166.28) | 116.72(±41.27) | 5.47(±2.63) | 4.1*(±5.34*) |

Table 3: Amari metrics for ICA algorithms in high dimensions. m is the dimension, reps is the number of replications, and N is the sample size

| m | reps | N | F-G0 | F-G1 | PICA | WICA | MICA | EICA |
|---|---|---|---|---|---|---|---|---|
| 4 | 100 | 1000 | 22.82(±16.69) | 27.98(±24.84) | 8.22(±7.34) | 52.11(±29.37) | 16.28(±9.07) | 25.94(±24) |
| 4 | 100 | 4000 | 11.03(±8.66) | 12.37(±11.85) | 4.28(±4.91) | 37.86(±22.83) | 7.34(±5.41) | 12.73(±14.57) |
| 8 | 50 | 2000 | 39.09(±25.19) | 42.44(±28.6) | 13.66(±11.98) | 120.41(±36.36) | 26(±9.8) | 39.35(±27.45) |
| 8 | 50 | 4000 | 25.2(±11.41) | 28.08(±19.16) | 7.79(±1.76) | 99.15(±27.37) | 16.07(±4.74) | 25.49(±18.1) |
| 16 | 25 | 2000 | 118.16(±29.06) | 111.62(±28.77) | 53.19(±39.23) | 309.51(±29.57) | 60.14(±15.57) | 102.37(±22.53) |
| 16 | 25 | 4000 | 61.35(±10.91) | 70.33(±21.45) | 17.61(±1.42) | 267.38(±28.37) | 37.3(±4.96) | 58.96(±14.32) |

## 2 Details of experiments with real data

Page 4, Column2, Section IV, Subsection C
The original images and recovered images are plotted in Figure 2.

Table 4: CPU elapsed time (ms) for ICA algorithms in high dimensions. m is the dimension, reps is the number of replications, and N is the sample size

| m | reps | N | F-G0 | F-G1 | PICA | WICA | MICA | EICA |
|---|---|---|---|---|---|---|---|---|
| 4 | 100 | 1000 | 54.25(±20.76) | 47.12(±15.14) | 4112.41(±1166.51) | 13.95(±7.91) | 302.52(±89.1) | $10^*(\pm 0^*)$ |
| 4 | 100 | 4000 | 214.62(±85.41) | 164.54(±66.21) | 6373.6(±2616.8) | 242.57(±62.35) | 359.83(±145.28) | $10^*(\pm 0^*)$ |
| 8 | 50 | 2000 | 218.5(±29.37) | 172.78(±22.36) | 11681.34(±1402.03) | 62.44(±51.3) | 636.94(±56.09) | $20^*(\pm 0^*)$ |
| 8 | 50 | 4000 | 444.8(±110.54) | 293.68(±79.85) | 12115(±3489.61) | 229.88(±88.4) | 750.5(±165.15) | $30^*(\pm 0^*)$ |
| 16 | 25 | 2000 | 563.2(±131.68) | 414.24(±75.91) | 27755.8(±4026.31) | 76.72(±18.64) | 1154.6(±26.73) | $80^*(\pm 0^*)$ |
| 16 | 25 | 4000 | 1020.8(±325.49) | 742.52(±250.03) | 30276.4(±9758.36) | 236.28(±91.03) | 1412.04(±78.95) | $80^*(\pm 0^*)$ |

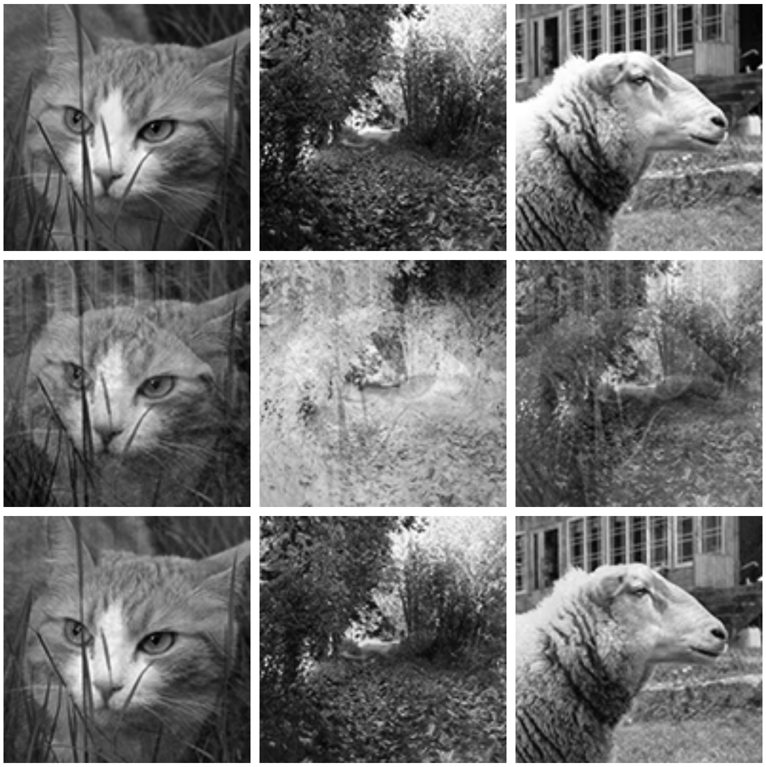

Figure 2: Recovery of image sources by $MDIICA$. From the top row to the bottom row, original sources, mixtures and recovered sources are plotted.
